# Supplementary material for: Discourse Probing of Pretrained Language Models
Source: arXiv:2104.05882 source file (2021-04-13)
Supplement: Supplementary file 1 [file dissent_appendix.pdf]

| ENGLISH |
|---|
| **Train**:<br>but: 2237, and: 2190, as: 1547, when: 1085, if: 993, before: 462, while: 358, because: 335, though: 229, after: 196, so: 180, although: 84, still: 38, then: 35, also: 31<br><br>**Development**:<br>but: 222, and: 192, as: 181, when: 116, if: 104, because: 44, before: 40, while: 28, though: 28, so: 16, after: 16, also: 5, although: 5, then: 2, still: 1<br><br>**Test**:<br>and: 211, but: 202, as: 153, when: 129, if: 97, before: 48, while: 44, because: 41, after: 20, though: 19, although: 11, so: 9, still: 7, also: 5, then: 4 |
| **CHINESE** |
| **Train**:<br>*other*: 520, 并: 182, 其中: 131, 也: 118, 但: 60, 而: 60, 还: 55, 以: 47, 使: 43, 后: 42, 为: 41, 同时: 37, 由于: 34, 因此: 28, 如: 26, 又: 20, 为了: 19, 如果: 17, 而且: 16, 但是: 15, 因为: 15, 虽然-但: 13<br><br>**Development**:<br>*other*: 22, 并: 7, 也: 6, 而: 6, 其中: 4, 但: 4, 因为: 4, 为: 3, 还: 3, 而且: 3, 又: 2, 如果: 2, 同时: 2, 使: 2, 后: 2, 如: 1, 由于: 1, 虽然-但: 1, 为了: 1<br><br>**Test**:<br>*other*: 60, 其中: 18, 并: 18, 也: 10, 使: 10, 还: 9, 同时: 8, 而: 6, 以: 5, 但: 5, 为: 4, 又: 3, 因为: 2, 虽然-但: 2, 由于: 2, 为了: 2, 因此: 2, 而且: 1, 如: 1 |
| **GERMAN** |
| **Train**:<br>*other*: 336, und: 191, doch: 62, wenn: 56, aber: 56, denn: 36, dann: 23, auch: 23, sondern: 19, oder: 19, so: 18, also: 17, deshalb: 16, weil: 15, als: 13<br><br>**Development**:<br>*other*: 50, und: 32, doch: 12, wenn: 11, aber: 9, denn: 6, dann: 5, so: 5, auch: 5, oder: 4, deshalb: 3, weil: 3, sondern: 2, als: 1<br><br>**Test**:<br>*other*: 69, und: 23, doch: 11, aber: 10, denn: 9, wenn: 8, dann: 8, so: 4, weil: 4, auch: 4, sondern: 3, deshalb: 3, oder: 2, als: 1 |
