# Supplementary material for: Discourse Probing of Pretrained Language Models
Source: arXiv:2104.05882 source file (2021-04-13)
Supplement: Supplementary file 2 [file rel_appendix.pdf]

| ENGLISH |
| --- |
| elab: 7830, attr: 3041, list: 1957, same: 1390, cont: 1108, evid: 967, back: 931, cause: 685, eval: 588, purp: 560, temp: 526, cond: 326, comp: 299, mann: 225, summ: 222, topic: 204, prob: 153, text: 142 |
| **CHINESE** |
| 并列类: 4144, 解说类: 1630, 因果类: 1333, 转折类: 214 |
| **GERMAN** |
| reason: 267, interpretation: 232, elaboration: 204, joint: 203, background: 163, list: 138, concession: 125, antithesis: 123, conjunction: 117, condition: 116, circumstance: 113, e-elaboration: 111, cause: 101, evidence: 99, preparation: 87, evaluation-s: 80, contrast: 49, result: 46, evaluation-n: 38, purpose: 30, sequence: 29, restatement: 17, means: 11, disjunction: 10, summary: 9, solutionhood: 7, justify: 4, otherwise: 3, enablement: 2, unless: 1, motivation: 1 |
| **SPANISH** |
| elaboración: 625, preparación: 370, lista: 257, fondo: 178, unión: 168, medio: 135, resultado: 134, circunstancia: 122, propósito: 115, secuencia: 79, interpretación: 77, antítesis: 67, contraste: 61, causa: 57, evidencia: 49, condición: 47, concesión: 44, justificación: 39, same-unit: 33, solución: 26, motivación: 21, reformulación: 16, conjunción: 14, disyunción: 9, evaluación: 9, resumen: 8, capacitación: 5, alternativa: 3, unless: 2 |
