# Supplementary material for: Discourse Probing of Pretrained Language Models
Source: arXiv:2104.05882 source file (2021-04-13)
Supplement: Supplementary file 3 [file appendix.pdf]

## A Pre-trained Language Models

| Model        | Huggingface model          |
|--------------|----------------------------|
| BERT         | bert-base-uncased          |
| BERT (large) | bert-large-uncased         |
| RoBERTa      | roberta-base               |
| ALBERT       | albert-base-v2             |
| ELECTRA      | electra-base-discriminator |
| GPT-2        | gpt2                       |
| BART         | bart-base                  |
| T5           | t5-small                   |

Table 3: List of English pretrained language models.

| Language | Huggingface model              |
|----------|--------------------------------|
| Chinese  | bert-base-chinese              |
| German   | bert-base-german-dbmdz-uncased |
| Spanish  | bert-base-spanish-wwm-uncased  |

Table 4: List of non-English BERT models.

## B Data Construction, Examples, and Training Configuration

### B.1 Next Sentence Prediction

We use spaCy (<https://spacy.io/>) to obtain sentences, and ensure that the distractor options in the training set do not overlap with the test set. For all languages and models, the training configurations are similar: the maximum tokens in the context and the next sentence are 450 and 50, respectively. If the token lengths are more than this, we truncate the context from the beginning of the sequence, and truncate the next sentence at the end of the sequence. We concatenate context with each option, and perform binary classification.

Other training configuration details: learning rate = 1e-3, Adam epsilon = 1e-8, maximum gradient norm = 1.0, maximum epochs = 20, warmup = 10% of the training steps, patience for early stopping = 5 epochs.

### B.2 Sentence Ordering

In generating sentence ordering data, we also use spaCy (<https://spacy.io/>) to obtain sentences from the document. For all languages and models, the training configurations are similar where the maximum token of each sentence: 50, learning rate: 1e-3, Adam epsilon: 1e-8, maximum gradient

| #Sentence (context) | Total |
|---------------------|-------|
| 2                   | 2500  |
| 4                   | 2500  |
| 6                   | 2500  |
| 8                   | 2500  |
| Total               | 10000 |

Table 5: NSP data based on the number of sentences.

| Context                                                                                                                               |
|---------------------------------------------------------------------------------------------------------------------------------------|
| <b>s1:</b> The Eastern Star, mostly carrying elderly tourists, capsized on 1 June near Jianli in Hubei province.                      |
| <b>s2:</b> Just 14 of the 456 passengers and crew are known to have survived.                                                         |
| Options                                                                                                                               |
| <b>0:</b> The channel recently said its signal was carried by 22 satellites                                                           |
| <b>0:</b> That step has become a huge challenge for opposition candidates                                                             |
| <b>0:</b> Six men were convicted and then acquitted of the atrocity and no-one has since been convicted of involvement in the bombing |
| <b>1:</b> A search is continuing for eight people who remain missing.                                                                 |

Table 6: Example of English NSP data with 2-sentence context. 1 indicates the correct next sentence.

| #Sentence | Total |
|-----------|-------|
| 3         | 2000  |
| 4         | 2000  |
| 5         | 2000  |
| 6         | 2000  |
| 7         | 2000  |
| Total     | 10000 |

Table 7: Sentence ordering data based on number of sentence.

norm: 1.0, epoch: 20, warmup: 10% of the training steps, patience for early stopping: 10 epochs.

### B.3 Discourse Connective Prediction

As our Chinese and German dataset are extracted from discourse treebanks, the number of distinct connective words varies. For instance, in the Chinese discourse treebank, we find 246 unique connective words. To simplify this, we set the connective word to *OTHER* if a connective word frequency is less than 12.

For all languages and models, the training con-

| Context                                                                                                                                 |
|-----------------------------------------------------------------------------------------------------------------------------------------|
| <b>s0:</b> West Mercia Police said the police do not encourage members of the public to pursue their own investigations.                |
| <b>s1:</b> David John Poole, from Hereford, poses online as a 14-year-old girl and says he has been sent hundreds of explicit messages. |
| <b>s2:</b> He says his work has led to two arrests in four weeks.                                                                       |
| Correct order: 2–0–1                                                                                                                    |

Table 8: Example of English sentence ordering data

figurations are: maximum token length of each sentence = 50, learning rate =  $1e-3$ , Adam epsilon =  $1e-8$ , maximum gradient norm = 1.0, maximum epochs = 20, warmup = 10% of the training steps, patience for early stopping = 10 epochs.

#### B.4 RST-related Tasks

In Figure 7 and Figure 8, we present the distribution of nuclearity and relation labels in the 4 different discourse treebanks. The English treebank is significantly larger, with a strong preference for the NS (nuclear–satellite) relationship. Unlike other languages, the proportion of NN (nuclear–nuclear) relationships in the Chinese discourse treebank (CDTB) is the highest. We also notice that the relation label set in CDTB is the simplest, with only 4 labels.

Most of the training details for nuclearity and relation prediction are the same as for the NSP task, except we set the maximum token length of each sentence to 250. Particularly for EDU segmentation, we set the maximum token length in a document to 512.

#### B.5 Cloze Story Test

As discussed in Table 2, we use cloze story test version-1 (Mostafazadeh et al., 2016). Although version-2 (Sharma et al., 2018) is better in terms of story biases, the gold labels for the test set are not publicly available, which limited our ability to explore different layers of a broad range of pre-trained language models (due to rate limiting of test evaluation).

For the data split, we followed previous work (Liu et al., 2018) in splitting the development set into a training and validation set. We perform binary classification similar to the NSP task, by first merging all 4-sentence stories into a single text (context). We limit the context to a maximum of

| ENGLISH                                                                                                                                                                                                                                                                                                                                                                                                                                                                                                                                                                |
|------------------------------------------------------------------------------------------------------------------------------------------------------------------------------------------------------------------------------------------------------------------------------------------------------------------------------------------------------------------------------------------------------------------------------------------------------------------------------------------------------------------------------------------------------------------------|
| <b>Train:</b><br>but: 2237, and: 2190, as: 1547, when: 1085, if: 993, before: 462, while: 358, because: 335, though: 229, after: 196, so: 180, although: 84, still: 38, then: 35, also: 31<br><br><b>Development:</b><br>but: 222, and: 192, as: 181, when: 116, if: 104, because: 44, before: 40, while: 28, though: 28, so: 16, after: 16, also: 5, although: 5, then: 2, still: 1<br><br><b>Test:</b><br>and: 211, but: 202, as: 153, when: 129, if: 97, before: 48, while: 44, because: 41, after: 20, though: 19, although: 11, so: 9, still: 7, also: 5, then: 4 |
| CHINESE                                                                                                                                                                                                                                                                                                                                                                                                                                                                                                                                                                |
| <b>Train:</b><br>other: 520, 并: 182, 其中: 131, 也: 118, 但: 60, 而: 60, 还: 55, 以: 47, 使: 43, 后: 42, 为: 41, 同时: 37, 由于: 34, 因此: 28, 如: 26, 又: 20, 为了: 19, 如果: 17, 而且: 16, 但是: 15, 因为: 15, 虽然-但: 13<br><br><b>Development:</b><br>other: 22, 并: 7, 也: 6, 而: 6, 其中: 4, 但: 4, 因为: 4, 为: 3, 还: 3, 而且: 3, 又: 2, 如果: 2, 同时: 2, 使: 2, 后: 2, 如: 1, 由于: 1, 虽然-但: 1, 为了: 1<br><br><b>Test:</b><br>other: 60, 其中: 18, 并: 18, 也: 10, 使: 10, 还: 9, 同时: 8, 而: 6, 以: 5, 但: 5, 为: 4, 又: 3, 因为: 2, 虽然-但: 2, 由于: 2, 为了: 2, 因此: 2, 而且: 1, 如: 1                                                 |
| GERMAN                                                                                                                                                                                                                                                                                                                                                                                                                                                                                                                                                                 |
| <b>Train:</b><br>other: 336, und: 191, doch: 62, wenn: 56, aber: 56, denn: 36, dann: 23, auch: 23, sondern: 19, oder: 19, so: 18, also: 17, deshalb: 16, weil: 15, als: 13<br><br><b>Development:</b><br>other: 50, und: 32, doch: 12, wenn: 11, aber: 9, denn: 6, dann: 5, so: 5, auch: 5, oder: 4, deshalb: 3, weil: 3, sondern: 2, als: 1<br><br><b>Test:</b><br>other: 69, und: 23, doch: 11, aber: 10, denn: 9, wenn: 8, dann: 8, so: 4, weil: 4, auch: 4, sondern: 3, deshalb: 3, oder: 2, als: 1                                                                |

Figure 5: Discourse connective word distribution.

450 tokens, and each candidate sentence (as the story ending) is limited to 50 tokens. Other training details are the same as for the NSP task.

|                                                                                                                                  |
|----------------------------------------------------------------------------------------------------------------------------------|
| <b>ENGLISH</b>                                                                                                                   |
| <b>S1:</b> Two men nudged the door open.<br><b>S2:</b> Slipped into the room with him.                                           |
| <b>Connective word:</b> and                                                                                                      |
| <b>CHINESE</b>                                                                                                                   |
| <b>S1:</b> 目前，约有十五万家外商投资企业在中国银行开立帐户，<br><b>S2:</b> 二万多家获得中国银行的贷款支持。                                                              |
| <b>Connective word:</b> 其中                                                                                                       |
| <b>GERMAN</b>                                                                                                                    |
| <b>S1:</b> der mann bezahlte viele handwerker nicht<br><b>S2:</b> wurde voriges jahr zu einer mehrjährigen haftstrafe verurteilt |
| <b>Connective word:</b> und                                                                                                      |

Figure 6: Discourse connective – data examples

|                                                                                                                                          |
|------------------------------------------------------------------------------------------------------------------------------------------|
| <b>ENGLISH</b>                                                                                                                           |
| <b>Train:</b> NS: 10348, NN: 3853, SN: 2702<br><b>Development:</b> NS: 1195, NN: 407, SN: 341<br><b>Test:</b> NS: 1373, NN: 507, SN: 428 |
| <b>CHINESE</b>                                                                                                                           |
| <b>Train:</b> NN: 3133, NS: 1784, SN: 1242<br><b>Development:</b> NN: 432, NS: 219, SN: 158<br><b>Test:</b> NN: 188, NS: 107, SN: 58     |
| <b>GERMAN</b>                                                                                                                            |
| <b>Train:</b> SN: 752, NS: 733, NN: 407<br><b>Development:</b> NS: 116, SN: 106, NN: 67<br><b>Test:</b> NS: 150, SN: 133, NN: 72         |
| <b>SPANISH</b>                                                                                                                           |
| <b>Train:</b> NS: 1011, SN: 570, NN: 461<br><b>Development:</b> NS: 163, SN: 73, NN: 71<br><b>Test:</b> NS: 211, SN: 121, NN: 89         |

Figure 7: Nuclearity label distribution.

|                                                                                                                                                                                                                                                                                                                                                                                                                                                                                        |
|----------------------------------------------------------------------------------------------------------------------------------------------------------------------------------------------------------------------------------------------------------------------------------------------------------------------------------------------------------------------------------------------------------------------------------------------------------------------------------------|
| <b>ENGLISH</b>                                                                                                                                                                                                                                                                                                                                                                                                                                                                         |
| elab: 7830, attr: 3041, list: 1957, same: 1390, cont: 1108, evid: 967, back: 931, cause: 685, eval: 588, purp: 560, temp: 526, cond: 326, comp: 299, mann: 225, summ: 222, topic: 204, prob: 153, text: 142                                                                                                                                                                                                                                                                            |
| <b>CHINESE</b>                                                                                                                                                                                                                                                                                                                                                                                                                                                                         |
| 并列类: 4144, 解说类: 1630, 因果类: 1333, 转折类: 214                                                                                                                                                                                                                                                                                                                                                                                                                                              |
| <b>GERMAN</b>                                                                                                                                                                                                                                                                                                                                                                                                                                                                          |
| reason: 267, interpretation: 232, elaboration: 204, joint: 203, background: 163, list: 138, concession: 125, antithesis: 123, conjunction: 117, condition: 116, circumstance: 113, e-elaboration: 111, cause: 101, evidence: 99, preparation: 87, evaluation-s: 80, contrast: 49, result: 46, evaluation-n: 38, purpose: 30, sequence: 29, restatement: 17, means: 11, disjunction: 10, summary: 9, solutionhood: 7, justify: 4, otherwise: 3, enablement: 2, unless: 1, motivation: 1 |
| <b>SPANISH</b>                                                                                                                                                                                                                                                                                                                                                                                                                                                                         |
| elaboración: 625, preparación: 370, lista: 257, fondo: 178, unión: 168, medio: 135, resultado: 134, circunstancia: 122, propósito: 115, secuencia: 79, interpretación: 77, antítesis: 67, contraste: 61, causa: 57, evidencia: 49, condición: 47, concesión: 44, justificación: 39, same-unit: 33, solución: 26, motivación: 21, reformulación: 16, conjunción: 14, disyunción: 9, evaluación: 9, resumen: 8, capacitación: 5, alternativa: 3, unless: 2                               |

Figure 8: Relation label distribution.

## C Full Experimental Results

| Layer             | NSP         | Sent.<br>Ord. | Discourse<br>Conn. | Nuclearity  | Relation    | EDU<br>segment. | Cloze<br>ST. |
|-------------------|-------------|---------------|--------------------|-------------|-------------|-----------------|--------------|
| BERT (English)    |             |               |                    |             |             |                 |              |
| 1                 | 0.37        | 0.28          | 0.27               | 0.62        | 0.38        | 0.30            | 0.55         |
| 2                 | 0.45        | 0.28          | 0.30               | 0.64        | 0.41        | 0.43            | 0.60         |
| 3                 | 0.81        | 0.29          | 0.30               | 0.62        | 0.40        | 0.47            | 0.64         |
| 4                 | 0.95        | 0.32          | 0.36               | 0.65        | 0.44        | 0.52            | 0.61         |
| 5                 | 0.97        | 0.32          | 0.43               | 0.76        | 0.55        | 0.55            | 0.67         |
| 6                 | 0.97        | <b>0.34</b>   | 0.52               | 0.78        | 0.61        | <b>0.56</b>     | 0.71         |
| 7                 | 0.96        | 0.33          | 0.57               | 0.80        | 0.65        | 0.55            | 0.73         |
| 8                 | 0.97        | 0.31          | 0.58               | <b>0.81</b> | <b>0.66</b> | 0.54            | 0.73         |
| 9                 | 0.96        | <b>0.34</b>   | 0.58               | 0.80        | 0.65        | 0.52            | 0.74         |
| 10                | 0.97        | <b>0.34</b>   | 0.58               | 0.80        | 0.64        | 0.47            | 0.76         |
| 11                | 0.98        | 0.32          | <b>0.60</b>        | 0.79        | 0.62        | 0.45            | <b>0.77</b>  |
| 12                | <b>0.99</b> | 0.32          | 0.56               | 0.76        | 0.58        | 0.39            | 0.76         |
| RoBERTa (English) |             |               |                    |             |             |                 |              |
| 1                 | 0.77        | 0.29          | 0.47               | 0.73        | 0.55        | 0.67            | 0.72         |
| 2                 | 0.86        | 0.31          | 0.47               | 0.74        | 0.56        | <b>0.92</b>     | 0.73         |
| 3                 | 0.88        | 0.31          | 0.51               | 0.75        | 0.58        | 0.90            | 0.75         |
| 4                 | 0.94        | 0.34          | 0.51               | 0.77        | 0.59        | 0.87            | 0.76         |
| 5                 | <b>0.96</b> | 0.37          | 0.50               | 0.78        | <b>0.61</b> | 0.89            | 0.7          |
| 6                 | <b>0.96</b> | 0.38          | 0.52               | 0.78        | <b>0.61</b> | 0.86            | 0.79         |
| 7                 | <b>0.96</b> | <b>0.39</b>   | 0.53               | 0.78        | <b>0.61</b> | 0.84            | 0.82         |
| 8                 | 0.95        | 0.38          | <b>0.55</b>        | 0.78        | <b>0.61</b> | 0.86            | 0.86         |
| 9                 | 0.94        | 0.37          | 0.53               | <b>0.79</b> | <b>0.61</b> | 0.86            | 0.87         |
| 10                | 0.93        | 0.37          | <b>0.55</b>        | 0.78        | <b>0.61</b> | 0.88            | <b>0.86</b>  |
| 11                | 0.93        | 0.34          | 0.53               | 0.77        | 0.59        | 0.85            | 0.84         |
| 12                | 0.90        | 0.31          | 0.48               | 0.75        | 0.56        | 0.73            | 0.81         |
| ALBERT (English)  |             |               |                    |             |             |                 |              |
| 1                 | 0.37        | 0.30          | 0.27               | 0.62        | 0.40        | 0.47            | 0.59         |
| 2                 | 0.84        | <b>0.33</b>   | 0.34               | 0.64        | 0.44        | <b>0.54</b>     | 0.65         |
| 3                 | 0.91        | 0.31          | 0.33               | 0.64        | 0.45        | <b>0.54</b>     | 0.69         |
| 4                 | 0.93        | 0.32          | 0.38               | 0.66        | 0.46        | 0.50            | 0.68         |
| 5                 | 0.96        | 0.31          | 0.38               | 0.67        | 0.47        | 0.47            | 0.71         |
| 6                 | 0.97        | 0.30          | 0.39               | 0.67        | 0.48        | 0.44            | 0.73         |
| 7                 | 0.97        | 0.27          | 0.37               | 0.68        | 0.48        | 0.40            | 0.72         |
| 8                 | <b>0.98</b> | 0.26          | 0.41               | 0.68        | 0.49        | 0.33            | 0.72         |
| 9                 | 0.97        | 0.23          | 0.40               | 0.68        | 0.49        | 0.32            | 0.76         |
| 10                | <b>0.98</b> | 0.20          | 0.42               | 0.69        | 0.50        | 0.25            | 0.77         |
| 11                | <b>0.98</b> | 0.20          | 0.44               | 0.72        | 0.53        | 0.17            | 0.79         |
| 12                | <b>0.98</b> | 0.16          | <b>0.52</b>        | <b>0.80</b> | <b>0.62</b> | 0.11            | <b>0.84</b>  |
| ELECTRA (English) |             |               |                    |             |             |                 |              |
| 1                 | 0.86        | 0.04          | 0.46               | 0.72        | 0.54        | 0.39            | 0.71         |
| 2                 | 0.90        | 0.07          | 0.48               | 0.73        | 0.56        | 0.47            | 0.74         |
| 3                 | 0.90        | 0.05          | 0.47               | 0.73        | 0.55        | 0.45            | 0.74         |
| 4                 | 0.94        | 0.02          | 0.51               | 0.75        | 0.57        | 0.50            | 0.75         |
| 5                 | 0.96        | 0.03          | 0.52               | 0.77        | 0.59        | 0.52            | 0.76         |
| 6                 | <b>0.97</b> | 0.05          | 0.53               | 0.78        | 0.59        | <b>0.57</b>     | 0.76         |
| 7                 | 0.96        | 0.04          | 0.54               | 0.79        | 0.61        | 0.54            | 0.79         |
| 8                 | <b>0.97</b> | 0.05          | 0.56               | <b>0.80</b> | 0.63        | 0.50            | 0.81         |
| 9                 | <b>0.97</b> | 0.05          | 0.57               | <b>0.80</b> | 0.63        | 0.48            | 0.86         |
| 10                | <b>0.97</b> | <b>0.10</b>   | <b>0.58</b>        | <b>0.80</b> | <b>0.64</b> | 0.49            | 0.88         |
| 11                | <b>0.97</b> | 0.07          | <b>0.58</b>        | <b>0.80</b> | 0.63        | 0.52            | <b>0.89</b>  |
| 12                | 0.96        | 0.09          | 0.57               | 0.79        | 0.60        | 0.47            | 0.87         |

Table 9: Full results of BERT, RoBERTa, ALBERT, and ELECTRA. All is English.

| Layer                                        | NSP         | Sent.<br>Ord. | Discourse<br>Conn. | Nuclearity  | Relation    | EDU<br>segment. | Cloze<br>ST. |
|----------------------------------------------|-------------|---------------|--------------------|-------------|-------------|-----------------|--------------|
| GPT-2 (English)                              |             |               |                    |             |             |                 |              |
| 1                                            | 0.85        | 0.27          | 0.47               | 0.73        | 0.55        | 0.33            | 0.73         |
| 2                                            | 0.87        | 0.26          | 0.48               | 0.73        | 0.56        | 0.35            | 0.73         |
| 3                                            | 0.88        | 0.28          | 0.50               | 0.73        | 0.56        | 0.39            | 0.74         |
| 4                                            | 0.90        | 0.30          | 0.50               | 0.75        | 0.56        | 0.40            | 0.76         |
| 5                                            | 0.91        | 0.33          | <b>0.51</b>        | 0.75        | 0.58        | 0.41            | 0.76         |
| 6                                            | <b>0.93</b> | 0.33          | 0.53               | <b>0.77</b> | 0.59        | 0.41            | 0.76         |
| 7                                            | <b>0.93</b> | 0.34          | 0.50               | 0.76        | <b>0.60</b> | <b>0.42</b>     | 0.77         |
| 8                                            | <b>0.93</b> | 0.33          | <b>0.51</b>        | 0.76        | <b>0.60</b> | 0.41            | <b>0.78</b>  |
| 9                                            | 0.92        | 0.33          | <b>0.51</b>        | 0.76        | 0.59        | <b>0.42</b>     | 0.76         |
| 10                                           | 0.91        | 0.31          | 0.50               | 0.74        | 0.58        | 0.41            | 0.77         |
| 11                                           | 0.91        | 0.30          | 0.50               | 0.73        | 0.57        | 0.40            | 0.75         |
| 12                                           | 0.85        | 0.27          | 0.48               | 0.73        | 0.53        | 0.40            | 0.72         |
| BART (English); Layers 7–12 are the decoder. |             |               |                    |             |             |                 |              |
| 1                                            | 0.86        | 0.29          | 0.48               | 0.73        | 0.55        | 0.79            | 0.73         |
| 2                                            | 0.92        | 0.32          | 0.49               | 0.76        | 0.58        | <b>0.88</b>     | 0.76         |
| 3                                            | 0.95        | 0.36          | 0.50               | 0.77        | 0.59        | <b>0.88</b>     | 0.75         |
| 4                                            | 0.95        | 0.38          | 0.53               | 0.78        | 0.60        | 0.85            | 0.77         |
| 5                                            | <b>0.96</b> | 0.39          | 0.54               | 0.78        | <b>0.62</b> | 0.81            | 0.81         |
| 6                                            | 0.96        | <b>0.41</b>   | 0.52               | <b>0.80</b> | <b>0.62</b> | 0.61            | 0.79         |
| 7                                            | 0.93        | 0.31          | 0.50               | 0.76        | 0.59        | 0.09            | 0.75         |
| 8                                            | 0.94        | 0.38          | 0.53               | 0.79        | 0.61        | 0.23            | 0.76         |
| 9                                            | 0.95        | 0.40          | <b>0.55</b>        | 0.79        | 0.61        | 0.31            | 0.75         |
| 10                                           | 0.95        | 0.39          | 0.53               | <b>0.80</b> | <b>0.62</b> | 0.29            | 0.76         |
| 11                                           | 0.95        | 0.38          | 0.53               | 0.79        | 0.60        | 0.34            | 0.76         |
| 12                                           | 0.94        | 0.38          | 0.52               | 0.77        | 0.59        | 0.47            | <b>0.82</b>  |
| T5 (English); Layers 7–12 are the decoder.   |             |               |                    |             |             |                 |              |
| 1                                            | 0.76        | 0.27          | 0.40               | 0.70        | 0.51        | 0.27            | 0.70         |
| 2                                            | 0.80        | 0.30          | 0.43               | 0.74        | 0.54        | 0.37            | 0.72         |
| 3                                            | 0.82        | 0.31          | 0.45               | 0.75        | 0.55        | <b>0.40</b>     | <b>0.73</b>  |
| 4                                            | 0.83        | 0.33          | 0.46               | 0.76        | 0.57        | 0.38            | 0.72         |
| 5                                            | <b>0.87</b> | 0.33          | 0.44               | 0.76        | 0.58        | 0.32            | 0.72         |
| 6                                            | 0.86        | <b>0.34</b>   | 0.46               | <b>0.77</b> | <b>0.59</b> | 0.28            | 0.71         |
| 7                                            | 0.76        | 0.29          | 0.41               | 0.73        | 0.55        | 0.24            | 0.66         |
| 8                                            | 0.76        | 0.27          | 0.45               | 0.75        | 0.55        | 0.27            | 0.72         |
| 9                                            | 0.76        | 0.25          | <b>0.47</b>        | 0.76        | 0.56        | 0.26            | 0.71         |
| 10                                           | 0.73        | 0.22          | 0.45               | 0.75        | 0.55        | 0.21            | 0.71         |
| 11                                           | 0.70        | 0.22          | 0.44               | 0.73        | 0.54        | 0.11            | 0.72         |
| 12                                           | 0.68        | 0.21          | 0.42               | 0.73        | 0.52        | 0.00            | <b>0.73</b>  |

Table 10: Full results of GPT-2, BART, and T5. All is English.

| Layer   | NSP         | Sent.<br>Ord. | Discourse<br>Conn. | Nuclearity  | Relation    | EDU<br>segment. |
|---------|-------------|---------------|--------------------|-------------|-------------|-----------------|
| Chinese |             |               |                    |             |             |                 |
| 1       | 0.30        | 0.38          | 0.36               | 0.53        | 0.58        | 0.71            |
| 2       | 0.49        | 0.38          | 0.36               | 0.53        | 0.58        | 0.75            |
| 3       | 0.47        | 0.41          | 0.36               | 0.53        | 0.58        | 0.79            |
| 4       | 0.83        | 0.43          | 0.36               | 0.51        | 0.58        | 0.79            |
| 5       | 0.90        | 0.44          | 0.38               | 0.59        | 0.62        | 0.81            |
| 6       | 0.92        | 0.45          | 0.39               | 0.59        | 0.65        | 0.82            |
| 7       | 0.93        | <b>0.46</b>   | 0.40               | 0.64        | 0.67        | <b>0.84</b>     |
| 8       | 0.94        | 0.45          | 0.46               | <b>0.65</b> | 0.66        | 0.83            |
| 9       | 0.94        | 0.42          | 0.43               | 0.64        | 0.67        | 0.82            |
| 10      | 0.96        | 0.42          | <b>0.52</b>        | <b>0.65</b> | <b>0.68</b> | 0.83            |
| 11      | <b>0.97</b> | 0.42          | 0.51               | 0.64        | 0.66        | 0.81            |
| 12      | <b>0.97</b> | 0.41          | 0.44               | 0.63        | 0.65        | 0.78            |
| German  |             |               |                    |             |             |                 |
| 1       | 0.44        | 0.58          | 0.43               | 0.47        | 0.17        | 0.55            |
| 2       | 0.59        | 0.58          | 0.43               | 0.42        | 0.19        | 0.57            |
| 3       | 0.76        | 0.59          | 0.45               | 0.46        | 0.19        | 0.66            |
| 4       | 0.76        | 0.62          | 0.44               | 0.48        | 0.23        | 0.70            |
| 5       | 0.98        | 0.63          | 0.47               | 0.49        | 0.27        | 0.73            |
| 6       | 0.99        | 0.62          | 0.48               | 0.53        | 0.30        | 0.75            |
| 7       | <b>1.00</b> | <b>0.67</b>   | 0.48               | 0.58        | 0.34        | <b>0.77</b>     |
| 8       | 0.99        | 0.64          | 0.48               | <b>0.60</b> | <b>0.35</b> | 0.75            |
| 9       | 0.99        | 0.64          | 0.47               | 0.58        | <b>0.35</b> | 0.67            |
| 10      | <b>1.00</b> | 0.63          | 0.48               | <b>0.60</b> | 0.34        | 0.65            |
| 11      | <b>1.00</b> | 0.64          | <b>0.55</b>        | 0.58        | 0.27        | 0.60            |
| 12      | <b>1.00</b> | 0.62          | 0.54               | 0.59        | 0.34        | 0.61            |
| Spanish |             |               |                    |             |             |                 |
| 1       | 0.39        | 0.49          | —                  | 0.50        | 0.29        | 0.42            |
| 2       | 0.54        | 0.52          | —                  | 0.58        | 0.31        | 0.50            |
| 3       | 0.57        | 0.53          | —                  | 0.58        | 0.31        | 0.53            |
| 4       | 0.96        | 0.55          | —                  | 0.62        | 0.38        | 0.56            |
| 5       | 0.98        | 0.55          | —                  | 0.65        | 0.41        | 0.60            |
| 6       | 0.99        | 0.56          | —                  | 0.67        | 0.46        | 0.61            |
| 7       | 0.99        | 0.56          | —                  | 0.68        | 0.47        | 0.677           |
| 8       | <b>1.00</b> | 0.57          | —                  | 0.74        | 0.50        | <b>0.70</b>     |
| 9       | <b>1.00</b> | 0.58          | —                  | 0.76        | 0.49        | 0.65            |
| 10      | <b>1.00</b> | <b>0.58</b>   | —                  | <b>0.77</b> | 0.54        | 0.62            |
| 11      | <b>1.00</b> | 0.57          | —                  | <b>0.77</b> | <b>0.55</b> | 0.59            |
| 12      | <b>1.00</b> | 0.55          | —                  | 0.75        | 0.52        | 0.49            |

Table 11: Full results of BERT-base model for Chinese, German, and Spanish.

| Layer                | NSP         | Sent.<br>Ord. | Discourse<br>Conn. | Nuclearity  | Relation    | EDU<br>segment. | Cloze<br>ST. |
|----------------------|-------------|---------------|--------------------|-------------|-------------|-----------------|--------------|
| BERT-Large (English) |             |               |                    |             |             |                 |              |
| 1                    | 0.33        | 0.27          | 0.29               | 0.61        | 0.38        | 0.23            | 0.61         |
| 2                    | 0.53        | 0.26          | 0.35               | 0.63        | 0.40        | 0.29            | 0.63         |
| 3                    | 0.57        | 0.27          | 0.35               | 0.63        | 0.42        | 0.30            | 0.65         |
| 4                    | 0.61        | 0.29          | 0.36               | 0.64        | 0.43        | 0.40            | 0.63         |
| 5                    | 0.64        | 0.30          | 0.38               | 0.65        | 0.43        | 0.43            | 0.70         |
| 6                    | 0.83        | 0.32          | 0.39               | 0.65        | 0.44        | 0.45            | 0.66         |
| 7                    | 0.87        | 0.32          | 0.41               | 0.66        | 0.45        | 0.44            | 0.70         |
| 8                    | 0.95        | 0.31          | 0.40               | 0.66        | 0.45        | 0.44            | 0.72         |
| 9                    | 0.96        | 0.30          | 0.40               | 0.67        | 0.47        | 0.43            | 0.66         |
| 10                   | 0.96        | 0.32          | 0.42               | 0.67        | 0.47        | 0.49            | 0.71         |
| 11                   | 0.97        | 0.32          | 0.41               | 0.68        | 0.48        | 0.53            | 0.69         |
| 12                   | 0.97        | 0.33          | 0.49               | 0.77        | 0.57        | 0.57            | 0.70         |
| 13                   | 0.97        | 0.34          | 0.53               | 0.78        | 0.61        | 0.56            | 0.72         |
| 14                   | 0.97        | 0.34          | 0.57               | 0.81        | 0.65        | <b>0.59</b>     | 0.73         |
| 15                   | 0.97        | 0.35          | 0.61               | 0.81        | 0.67        | 0.58            | 0.74         |
| 16                   | 0.97        | 0.36          | 0.60               | <b>0.83</b> | 0.67        | 0.56            | 0.7          |
| 17                   | 0.97        | 0.35          | <b>0.63</b>        | <b>0.83</b> | <b>0.68</b> | 0.53            | 0.83         |
| 18                   | 0.98        | 0.34          | 0.62               | 0.82        | <b>0.68</b> | 0.53            | 0.82         |
| 19                   | <b>0.99</b> | <b>0.37</b>   | <b>0.63</b>        | 0.83        | 0.67        | 0.50            | 0.83         |
| 20                   | <b>0.99</b> | 0.34          | <b>0.63</b>        | 0.82        | 0.66        | 0.48            | <b>0.85</b>  |
| 21                   | <b>0.99</b> | 0.34          | <b>0.63</b>        | 0.81        | 0.65        | 0.40            | 0.84         |
| 22                   | <b>0.99</b> | 0.35          | 0.60               | 0.81        | 0.64        | 0.36            | 0.84         |
| 23                   | <b>0.99</b> | 0.34          | 0.60               | 0.80        | 0.63        | 0.35            | 0.83         |
| 24                   | <b>0.99</b> | 0.33          | 0.57               | 0.78        | 0.59        | 0.31            | 0.81         |

Table 12: Full results of English BERT-large.

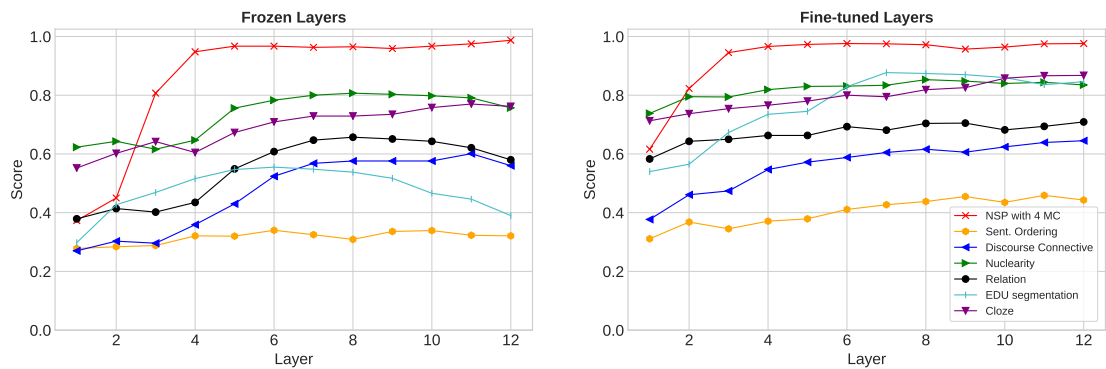

Figure 9

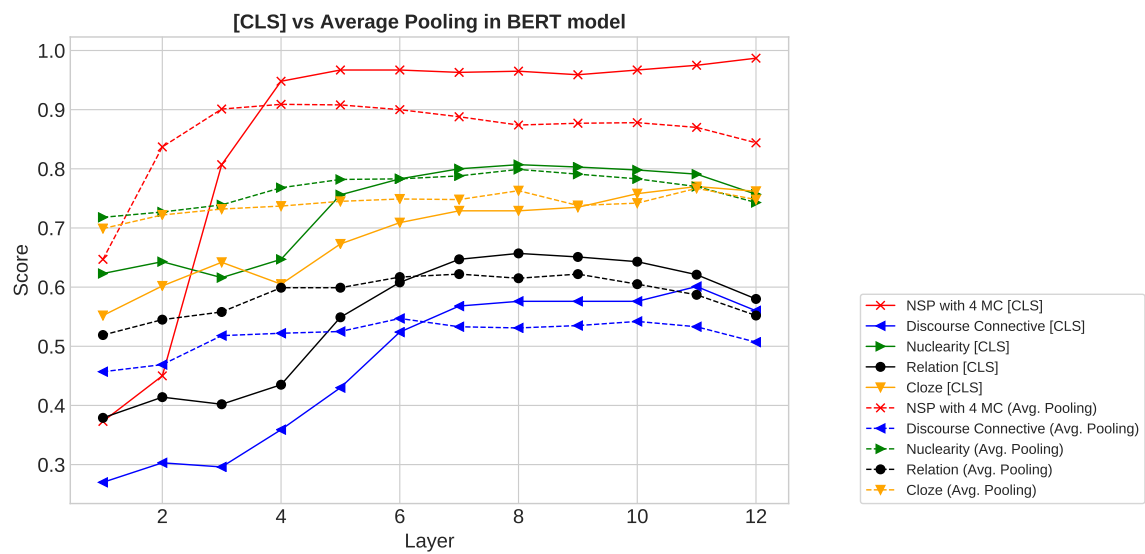

Figure 10
